# Supplementary material for: RNN-Test: Towards Adversarial Testing for Recurrent Neural Network Systems
Source: arXiv:1911.06155 source file (2021-01-08)
Supplement: Supplementary file 1 [file sec-appendix.tex]

% !TeX root = main_body.tex
\appendix
\section{Justification for Coverage Metrics}\label{sec:appendix}
We provide a simple illustration for coverage metrics here. As discussed in \S~\ref{sec:coverage}, Hidden state coverage is designed to measure prediction logics for each hidden state. Cell state coverage is designed to measure the logics of each cell state protecting context information.

\begin{figure}[h]
\centering
	\subfloat[Hidden state coverage]{\includegraphics[width=0.45\linewidth]{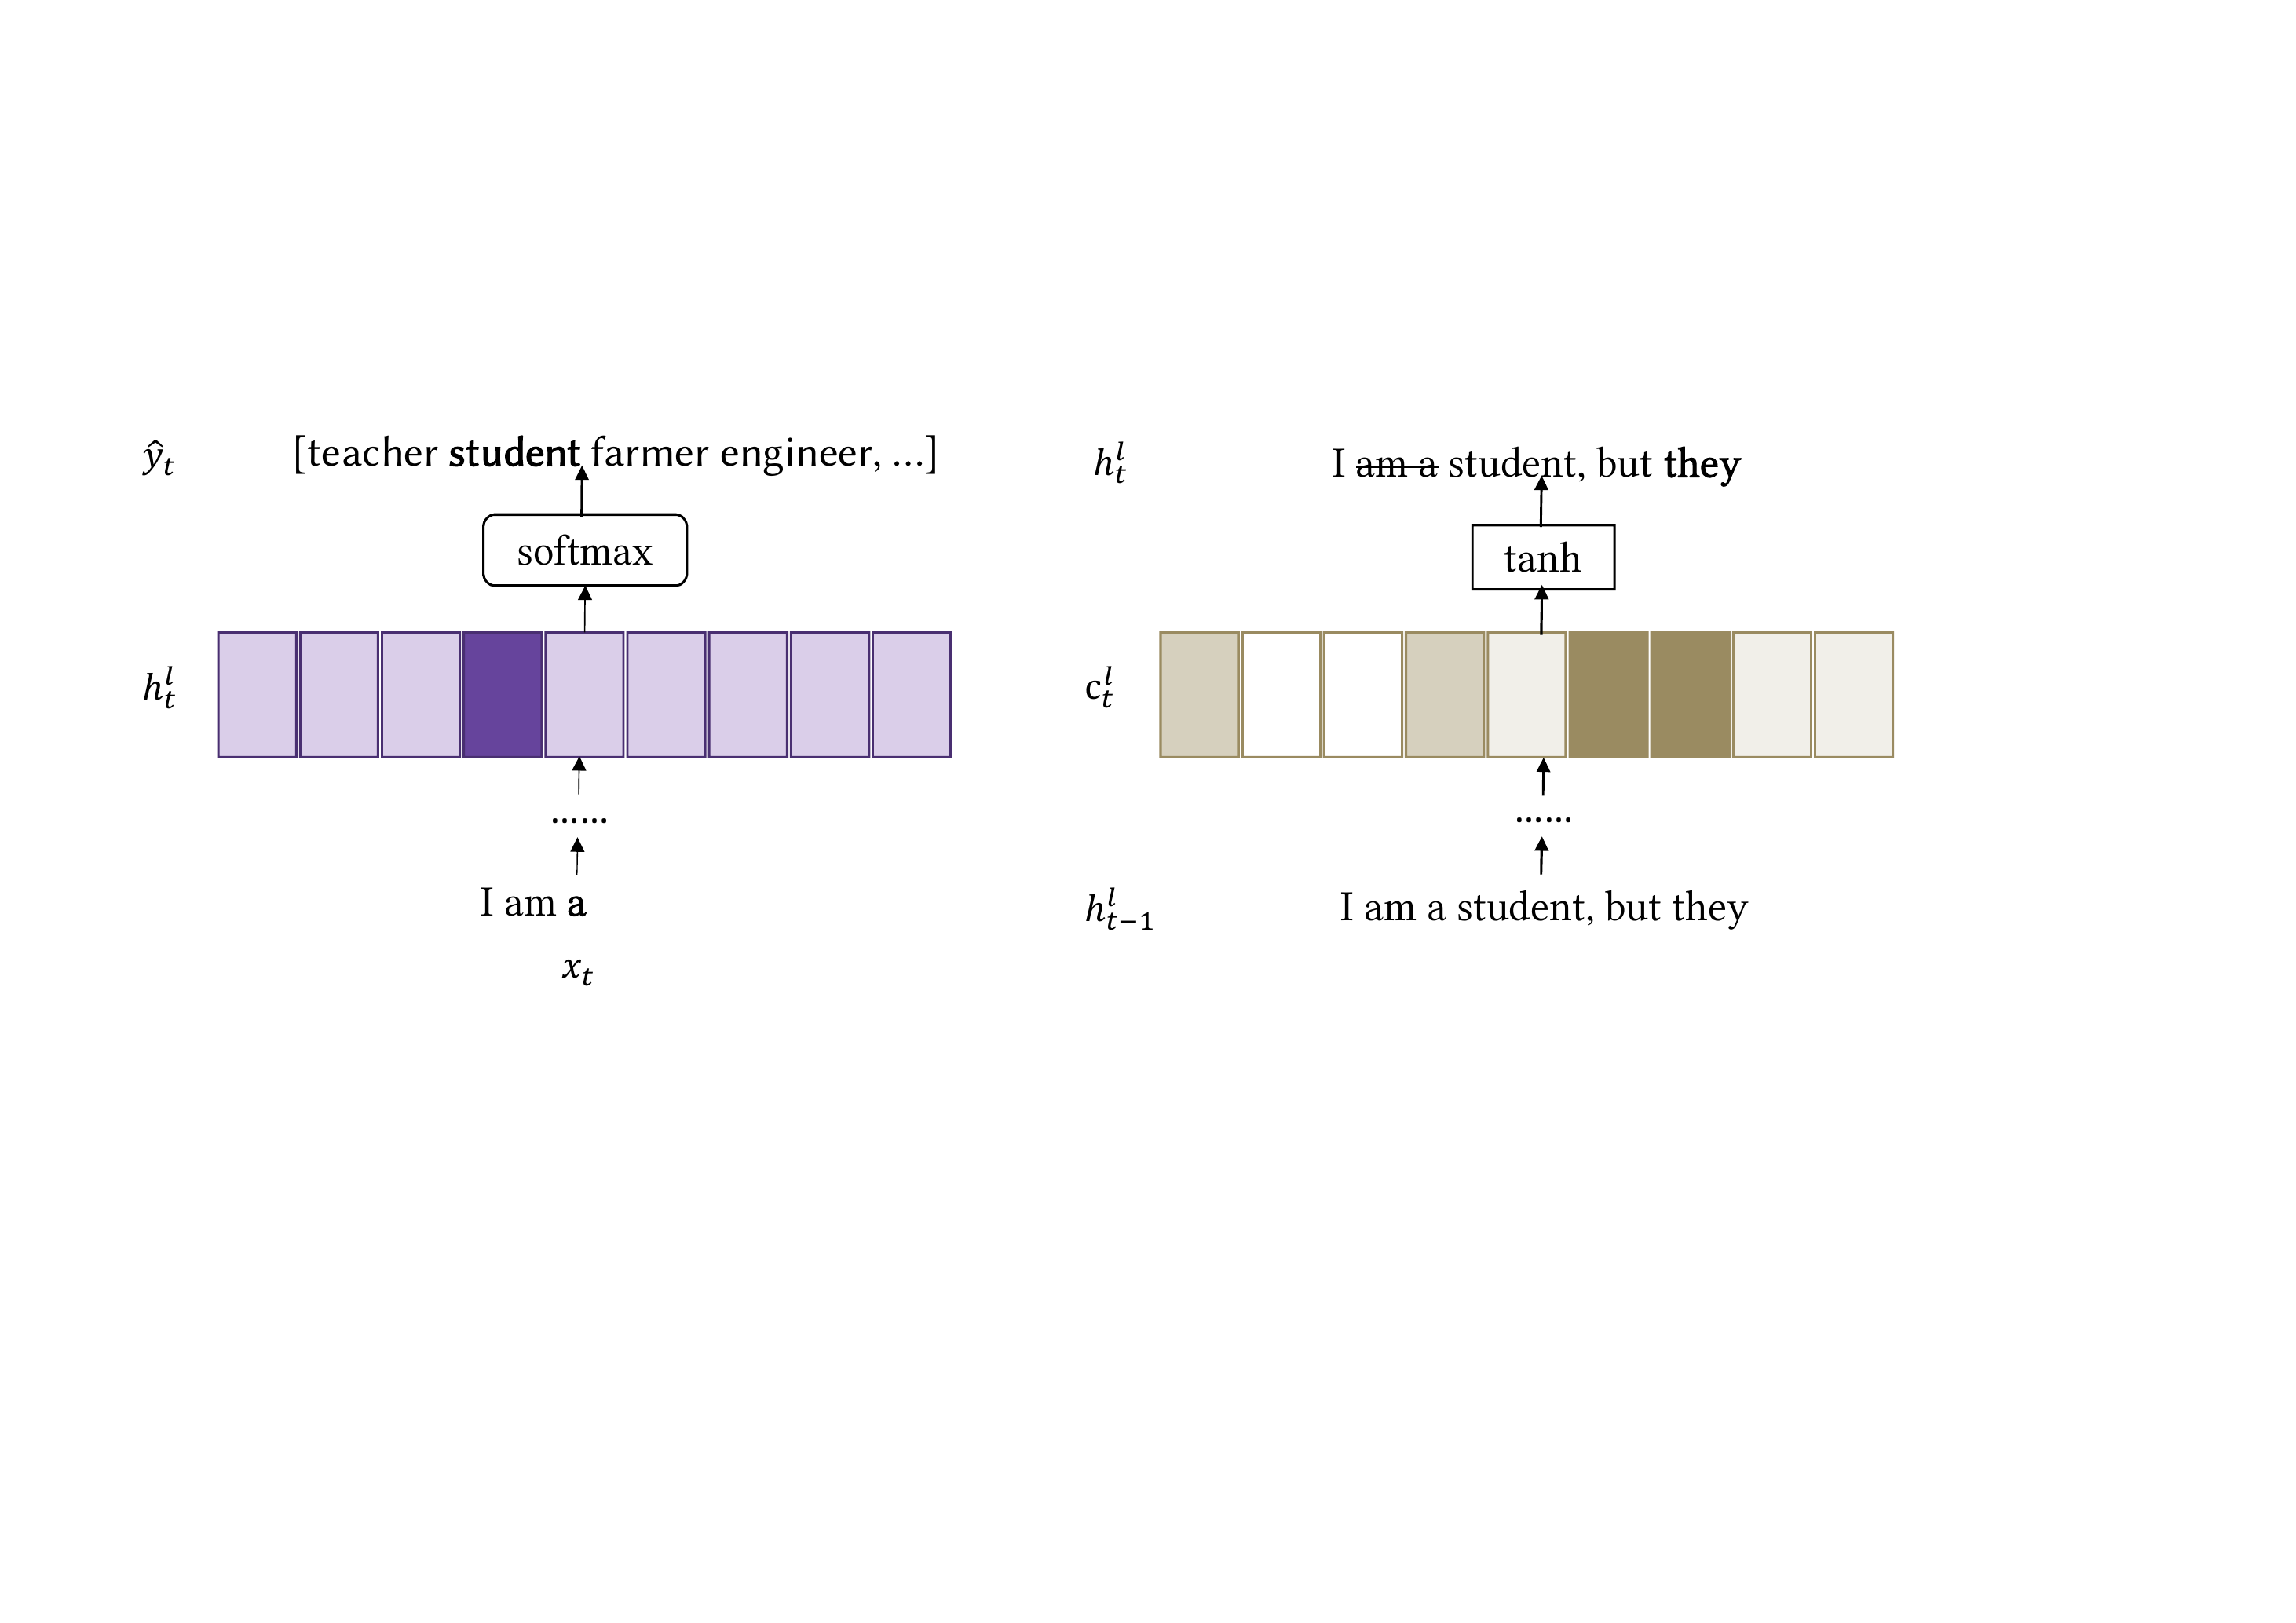}
     \label{fig:graph hs_c}}
     %\hspace{width=0.03\linewidth}
    \subfloat[Cell state coverage]{\includegraphics[width=0.45\linewidth]{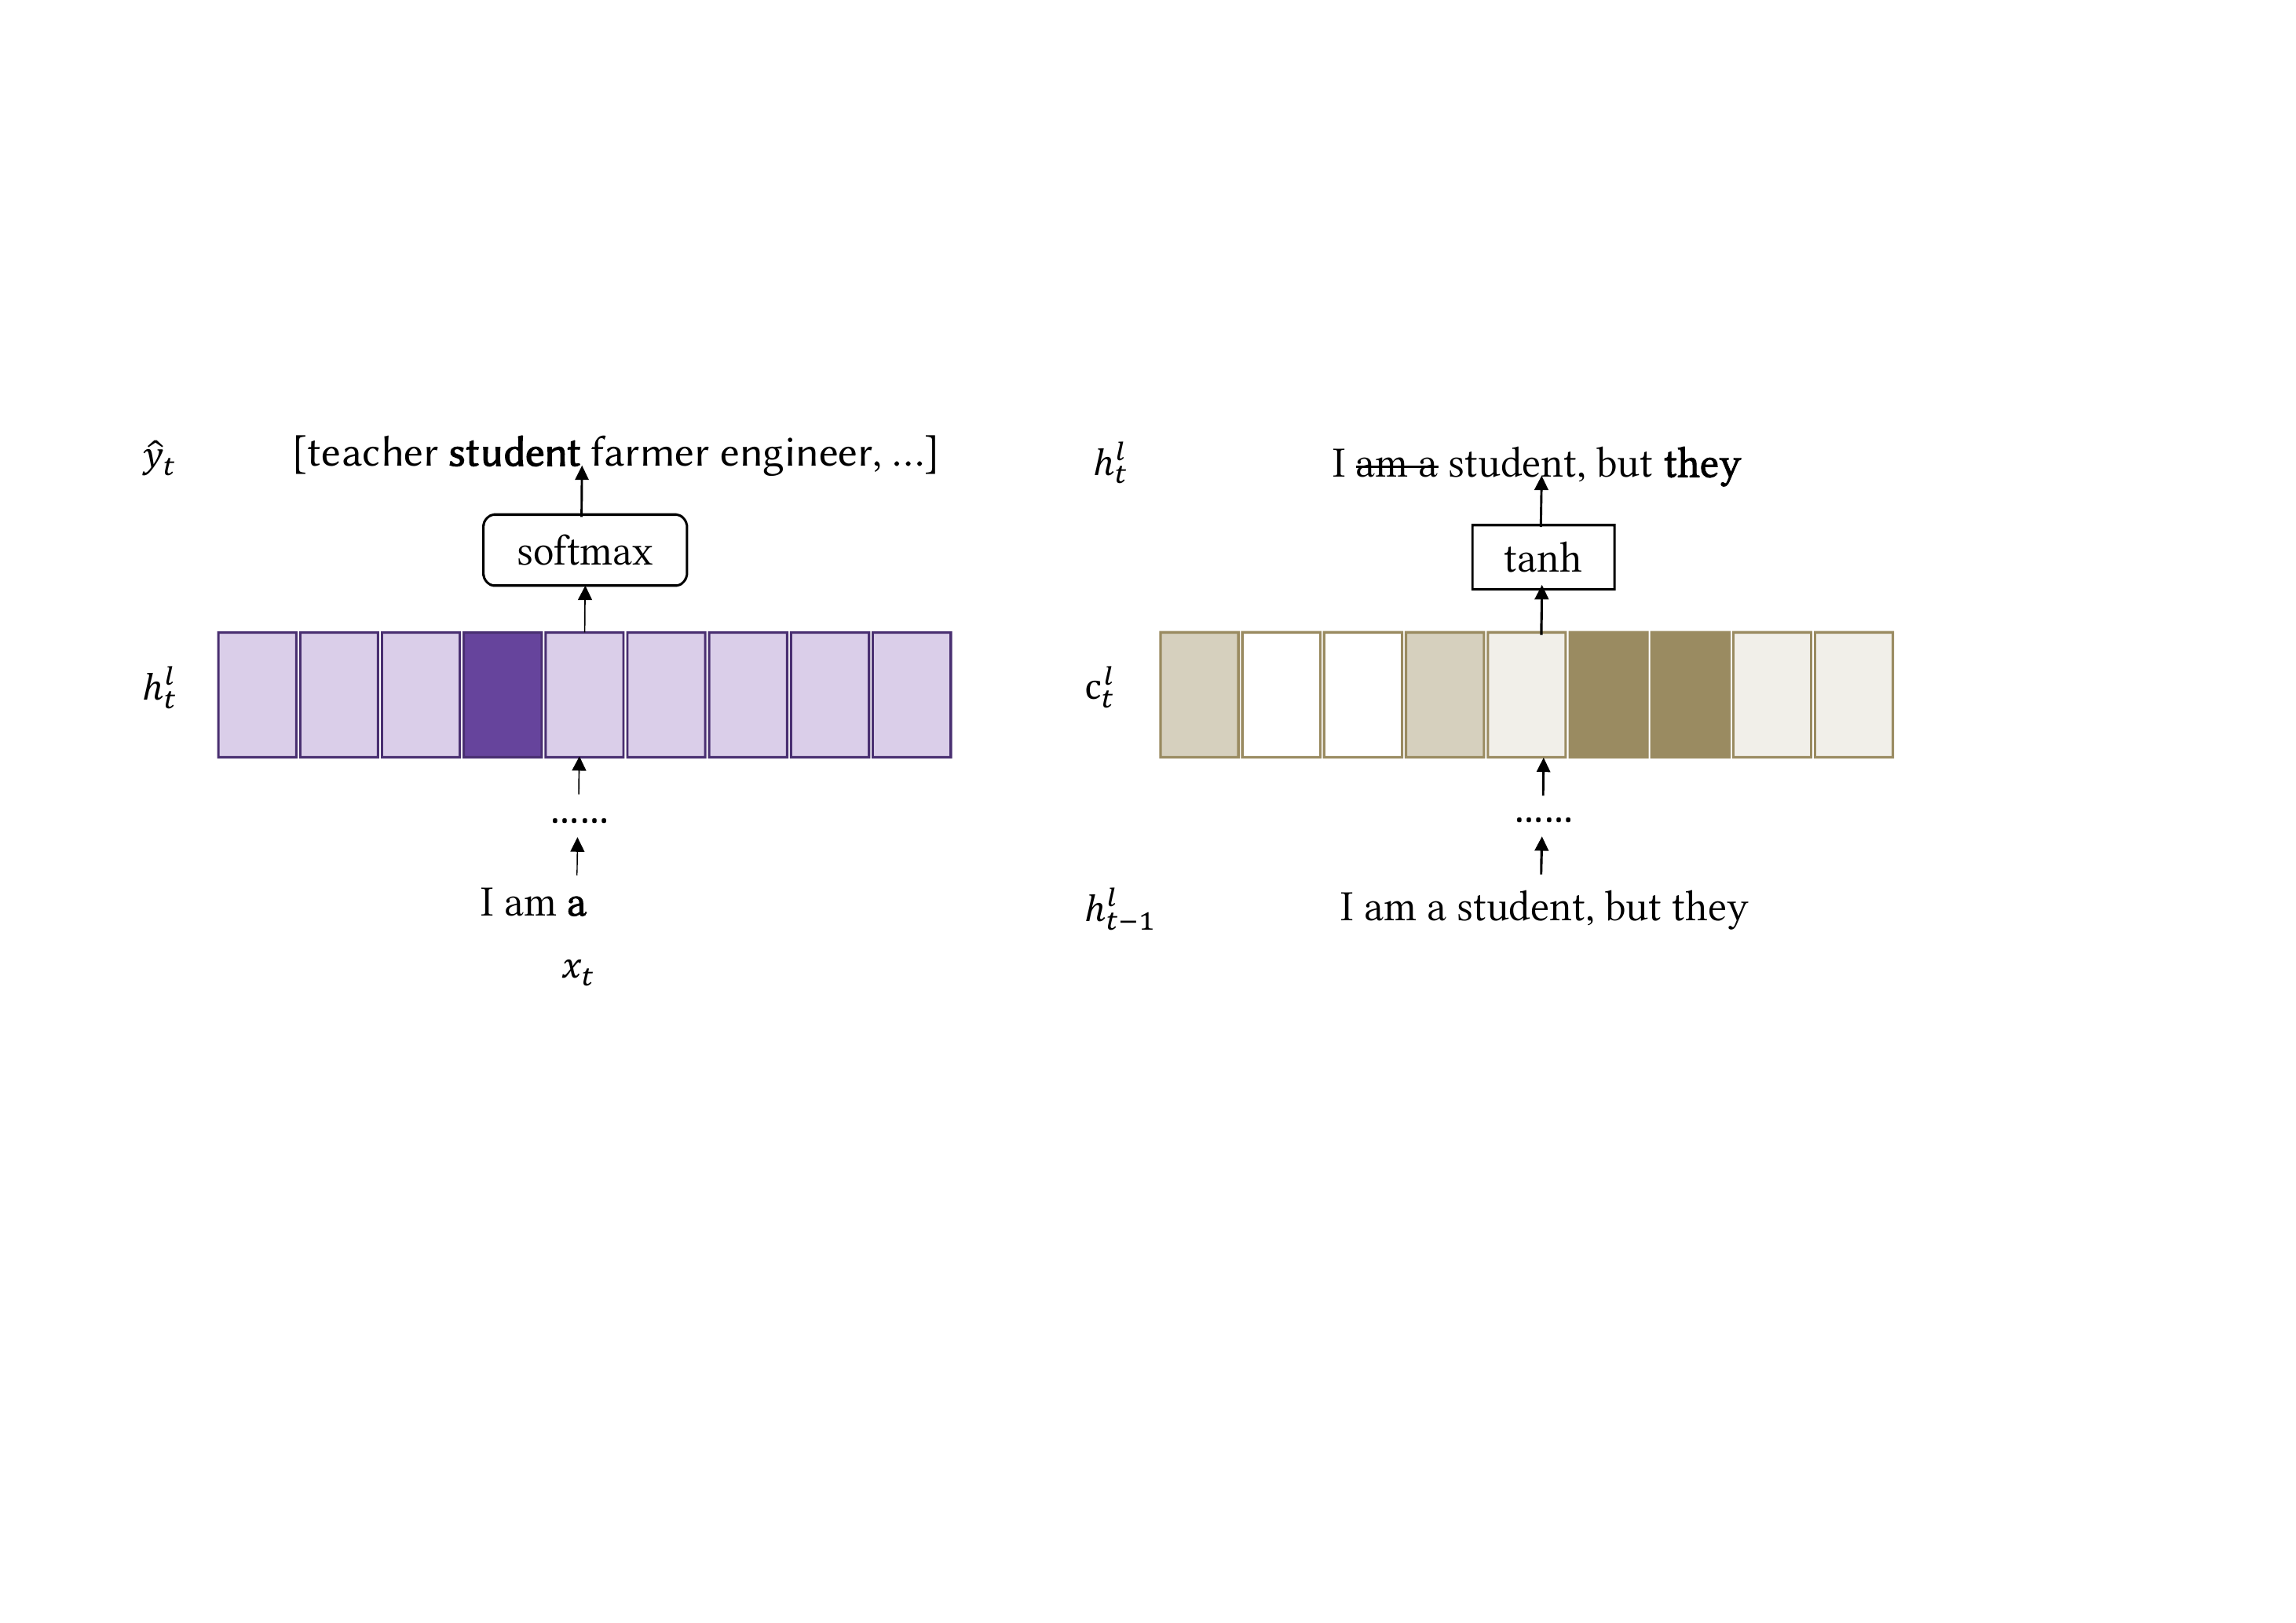}
     \label{fig:graph cs_c}}
\caption{A simple illustration for motivation of proposed coverage metrics. Each rectangle represents each hidden (or cell) state, where darker color means higher value.} 
\label{fig:coverage illustration}
\end{figure}

In Fig.~\ref{fig:coverage illustration}, $h_{t}^{l}$ and $c_{t}^{l}$ are the outputs of RNN cells, where they are both a vector containing many hidden (or cell) states. Thus, each rectangle represents each hidden (or cell) state, where darker color means higher value. In Fig.~\ref{fig:graph hs_c}, hidden states will be mapped to prediction result $\hat{y}_t$, a list of candidates for next word following $x_{t}$. If each hidden state is to be maximum, its mapped candidate~(e.g. student) will be of higher prediction probability. In Fig.~\ref{fig:graph cs_c} different value ranges of each cell state will result in different degrees of input semantics to keep, where we replace hidden states as a sentence to describe more clearly. If it is to predict the predicate after "they", context information of "am a" is supposed to be discarded and that of "they" need to be put more weights on. Based on these insights, our coverage metrics are accordingly designed.
